# Supplementary material for: Towards A Proactive ML Approach for Detecting Backdoor Poison Samples
Source: arXiv:2205.13616 source file (2023-06-18)
Supplement: Supplementary file 1 [file appendix_rather_few_clean_samples.tex]

\section{\revision{Confusion Training with Very Small Reserved Clean Dataset}}
\label{appendix:rather-few-clean-asmples}

\revision{Figure~\ref{fig:ablation_num_clean} presents our ablation study on the size of the reserved clean set. The study reveals that the TPR of our CT detection pipeline maintains a relatively robust performance, even as the number of reserved clean samples becomes smaller. However, a noticeable trade-off in the FPR becomes evident. Remarkably, when the quantity of reserved clean samples is reduced to 250, the FPR can, at times, exceed $20\%$, leading to a substantial loss of training data.}

\input{sections/tables/table_few_clean}

\revision{To better understand how this level of sacrifice in the training sample affects the overall performance of our defense, we also report the ACC and ASR for this ablation study. We focus on the hardest case where we only possess 250 clean samples to bootstrap CT for CIFAR10. We measure the ACC and ASR by retraining ResNet18 on the cleansed dataset, adhering to the same practice specified in Section~\ref{subsubsec:exp_setup}. We present the results in Table~\ref{tab:ct-few-clean}. Intriguingly, we see that CT maintains an impressive ACC, exceeding $91\%$ in all cases. This is achieved even at the sacrifice of over $20\%$ of the CIFAR10 training set against Adap-Blend. Simultaneously, the high TPR that we continue to have ensures that the ASR remains low.}

\revision{This result has interesting practical implications, suggesting that for datasets of adequate size, a relatively high FPR could be tolerated during dataset cleansing operations. The remaining data has the potential to continue to suffice for the training of a high-quality model. A closely relevant research topic to this observation is Dataset Pruning~\cite{paul2021deep}, which shows that many training data can be removed from the dataset while models trained on the remaining dataset can still be accurate.} 
%potentially continue to suffice for the training of a highly accurate model.}
