# Supplementary material for: Towards A Proactive ML Approach for Detecting Backdoor Poison Samples
Source: arXiv:2205.13616 source file (2023-06-18)
Supplement: Supplementary file 2 [file appendix_related_work.tex]

\section{A More Detailed Review of Backdoor Attacks on Neural Networks}
\label{appendix:backdoor_attacks_on_neural_networks}

Deep neural network~(DNN) models are susceptible to backdoor attacks~\cite{li2022backdoor}. A DNN model is said to be backdoored, if: (1) the model has been embedded a certain backdoor rule that is exclusively known to the adversary; (2) the model still behaves normally under standard evaluations. Specifically, the backdoor rule is typically a malicious correlation between a backdoor trigger~(certain pattern) and a target prediction, which is specified by the adversary. The backdoor rule is often dominant, to an extent that the backdoored model will mispredict trigger-planted samples to the target prediction~(i.e. achieve high attack success rate) based on the backdoor rule, regardless of their clean semantics that really determine the ground-truth. Moreover, the backdoor rule is hidden --- on clean samples that do not contain the backdoor trigger, the backdoored model just behaves as normal as a benign model~(i.e. preserve high clean accuracy). 
Backdoor attacks involve a range of prototypes with different threat models. We divide them into two families: 1) {backdoor poisoning attacks} that this work aims to defend against and 2) {other attacks} that do not fit into our threat model.

\textbf{Backdoor Poisoning Attacks.}  The primary focus of this study is to address the threat of \textit{backdoor poisoning attacks} on deep neural networks (DNNs), which are the most prevalent form of DNN backdoor attacks. These attacks~\cite{gu2017badnets,Chen2017TargetedBA,liu2017trojaning,turner2019label,barni2019new,severi2020exploring,nguyen2020input,li2021invisible,nguyen2021wanet,liu2020reflection,li2021invisible,tang2021demon,qi2023revisiting,wu2022just} involve the manipulation of a few samples in the training dataset by an attacker, resulting in the "poisoning" of the dataset. The victim will then train her own model on this poisoned dataset and inadvertently get a backdoored model.

The earliest forms of backdoor poisoning attacks~(e.g., \cite{gu2017badnets,Chen2017TargetedBA,liu2017trojaning}) fall under the subcategory of \textit{dirty label attacks}. In these attacks, the adversary alters a small number of samples in the victim's training dataset by planting a backdoor trigger and mislabeling them as a specific target class. These manipulated samples, referred to as backdoor poison samples, establish a backdoor correlation between the trigger and the target class. As a result, models trained on the poisoned dataset inadvertently learn this backdoor correlation, becoming vulnerable to the attack.

To enhance stealthiness against human inspections, \textit{clean label attacks}~\cite{turner2019label,barni2019new,severi2020exploring} propose to avoid mislabeling poison samples and instead only plant the trigger in samples that are originally from the target class. Other efforts to enhance stealthiness include using different triggers for different poison samples~(i.e., \textit{sample specific attacks}~\cite{nguyen2020input,li2021invisible}), investigating triggers that are hard to notice~\cite{liu2020reflection,li2021invisible}, and studying adaptive backdoor poisoning attacks~\cite{tang2021demon,qi2023revisiting} that are stealthy in the latent representation space.

To our best knowledge, {backdoor poisoning attacks} are first demonstrated by \citet{gu2017badnets}. They randomly select a small number of samples from the training dataset, stamp them with a fixed patch pattern and mislabel them to a target class, and observe that models trained on such datasets consistently learn a dominant backdoor correlation between the patch pattern and the target class.

For example, in a typical backdoor poisoning attack, the adversary will modify a small portion of the victim's training samples by adding a backdoor trigger~(e.g. a specific pixel patch) to them and (mis)label them to a specific target class. This manipulation will create an artificial correlation between the trigger pattern and the target class. Models that fit these manipulated samples~(i.e. poison samples) will thus learn this adversarially created correlation~(i.e. learn a backdoor). Backdoor poisoning attacks are considerably risky, because those backdoored models behave almost the same as normal models under standard evaluation metrics but can make catastrophic mistakes stealthily controlled by adversaries.

Backdoor poisoning attacks only require manipulations on a small number of samples in the victim's training dataset, which are intrinsically challenging to prevent due the automatic collection procedure, intensive third-party involvement as well as the large scale of modern datasets.

Subsequent work further propose different poison strategies for further improving the practicality of the attacks. These improvements include different types of triggers~\cite{Chen2017TargetedBA, nguyen2020input}, clean label attacks~\cite{turner2019label,barni2019new}, adaptive attacks~\cite{qi2023revisiting} that can evade certain defenses, etc.

In order to improve the practicality of backdoor poisoning attacks, subsequent work in this line further propose different poison strategies. For example, \citet{Chen2017TargetedBA} suggest image blending between clean images and trigger image as an effective way for crafting backdoor poison samples. \citet{turner2019label} further propose the concept of clean label attacks~(also known as label-consistent attacks), which only manipulate samples from the target class. Similarly, \citet{barni2019new} also find that using sinusoidal signal as backdoor triggers can enable cean label attacks.  \citet{nguyen2020input} relax the restriction of fixed trigger pattern and propose to use dynamic input-specific trigger patterns. 

\textbf{Other Backdoor Attacks.} The literature on backdoor attacks includes various methods that do not fit within the paradigm of data poisoning. Examples include modifying the training process~\cite{bagdasaryan2021blind,tan2019bypassing} or using backdoored pre-trained models~\cite{yao2019latent,shen2021backdoor} for transfer learning, as well as attacks that occur at the deployment stage~\cite{liu2017fault,qi2021towards,rakin2020tbt}. These attacks involve different assumptions and threat models, which are out of the scope of this work. For a more comprehensive overview, readers are referred to \citet{li2022backdoor}.
