# Supplementary material for: Towards A Proactive ML Approach for Detecting Backdoor Poison Samples
Source: arXiv:2205.13616 source file (2023-06-18)
Supplement: Supplementary file 3 [file appendix_visualization.tex]

\section{Visualization of Latent Representation Space}
\label{appendix:visualization_of_latent_space}

In this section, we present our full visualization results of latent representation space on CIFAR10, for a set of backdoored models attacked by different poison strategies. 

\paragraph{Procedure of The Visualization.} For each poison strategy, we first construct the resulting poisoned dataset following the configuration in Appendix~\ref{appendix_subsec:details_baseline_attacks}. Then, we train a backdoored model on this poisoned dataset with a standard training~(see Appendix~\ref{appendix_subsec:details_training_backdoored_models}). Next, we take out all samples that are \textbf{labelled as the target class} from the poisoned set and use the trained backdoored model to project them into the latent representation space. Finally, for visualization purpose, we project these latent representations to low dimensional visual planes.

\paragraph{PCA~\cite{pearson1901liii} Projection.} In Figure~\ref{fig:vis_latent_space_compare} that we present in the main text, we use PCA~\cite{pearson1901liii} to project these latent representations into the top-2 principal directions. In Figure~\ref{fig:vis_latent_space_compare_repeat}, we present the full results produced by PCA projection, where the experiments are repeated for three times.

\paragraph{t-SNE~\cite{van2008visualizing} Projection.} Considering that PCA may not well capture the local similarity structure, alternatively, we also use t-SNE~\cite{van2008visualizing}, which is designed specifically for preserving local structure and arguably one of the best dimensionality reduction technique. In Figure~\ref{fig:vis_latent_space_compare_repeat_tsne}, we present the visualization results with two-dimensional t-SNE projection. 

\paragraph{Oracle Projection.} Note that, both PCA and t-SNE are unsupervised methods for discovering structures. The low dimension projection generated by these two methods may still not faithfully reflect the real extent of separation between poison and clean samples --- these unsupervised dimensionality reduction methods may only keep other irrelevant structures and throw the information about the separability. Thus, following the same practice in \citet{qi2022circumventing}, we also incorporate oracle knowledge~(in the experimental simulation, we know which one is poison and which one is not) about poison and clean samples to improve the visualization. Specifically, we model the problem of poison samples detection as a binary classification problem, where poison samples form the positive class and clean samples form the negative class. Then, we use Support Vector Machine~(SVM) to fit these samples. Intuitively, the fitted hyperplane by SVM is the approximately optimal linear boundary between the two classes. Finally, we compute the (signed) distance between each point and the fitted hyperplane, and plot the distance histogram in Figure~\ref{fig:vis_latent_space_compare_repeat_oracle}. Conceptually, if the poison and clean populations are very well separated in the latent representation space, then the two groups should stay in the opposite side of the SVM hyperplane, and thus the distance histograms of these two different groups will also be far well separated. This is true for the naive BadNet~(Figure~\ref{fig:vis_badnet_repeat_oracle}). However, \textbf{for adaptive poison strategies, one can see~(Figure~\ref{fig:vis_adaptive_blend_repeat_oracle},\ref{fig:vis_adaptive_k_repeat_oracle}) that even with oracle knowledge, it is hard to separate the two groups with a linear boundary}.

\input{sections/assets/visualization_latent_compare_repeat}
\input{sections/assets/visualization_latent_compare_repeat_tsne}
\input{sections/assets/visualization_latent_compare_repeat_oracle}
