# Supplementary material for: Towards A Proactive ML Approach for Detecting Backdoor Poison Samples
Source: arXiv:2205.13616 source file (2023-06-18)
Supplement: Supplementary file 4 [file appendix_light_weight_detector_for_heavy_weight_model.tex]

\section{\revision{Using Lightweight Poison Detector to \\Safeguard Heavyweight Models}}
\label{appendix:lightweight_for_heavy}

xxx
